# Supplementary material for: Local flow measurements around flexible filaments under rotating magnetic field
Source: arXiv:2307.02228 source file (2023-07-05)
Supplement: Supplementary file 1 [file Stikuts-et-al-Local_flow_measurements_Supplementary_information.pdf]

# Local flow measurements around flexible filaments under rotating magnetic field
# Supplementary information


Andris Pāvils Stikuts, Abdelqader Zaben, Ivars Driķis, Māra Šmite, Rūdolfs Livanovičs, Andrejs Cēbers, Guntars Kitenbergs

MMML lab, Department of Physics, University of Latvia,
Riga, Jelgavas 3, LV1004, Latvia;
e-mail: guntars.kitenbergs@lu.lv


## 1 Calculated velocity field around a straight rotating rod

The calculation of the velocity field around a straight rotating rod was done in Wolfram Mathematica and the respective calcuation is given in the supplementary materials as the Wolfram Mathematica notebook.

## 2 Parameters for filaments in experiments and simulations

<table>
<tr><th>filament</th><th>beads</th><th>$L, \mu$m</th><th>$f$, Hz</th><th>$B_{ext}$ or $\mu_0 H$, mT</th><th>$a, \mu m$</th><th>$A, J \cdot m$</th><th>$M, A \cdot m$</th><th>$\eta, Pa \cdot s$</th></tr>
<tr><td rowspan="5">0</td><td rowspan="5">17</td><td rowspan="5">72.4</td><td>1</td><td rowspan="18">3.44</td><td rowspan="18">2.13</td><td rowspan="18">$2.7 \cdot 10^{-21}$</td><td rowspan="18">$3.3 \cdot 10^{-8}$</td><td rowspan="18">$1 \cdot 10^{-3}$</td></tr>
<tr><td>2</td></tr>
<tr><td>3</td></tr>
<tr><td>4</td></tr>
<tr><td>5</td></tr>
<tr><td rowspan="3">1</td><td rowspan="3">14</td><td rowspan="3">59.6</td><td>1</td></tr>
<tr><td>2</td></tr>
<tr><td>3</td></tr>
<tr><td rowspan="5">2</td><td rowspan="5">11</td><td rowspan="5">46.9</td><td>1</td></tr>
<tr><td>2</td></tr>
<tr><td>3</td></tr>
<tr><td>4</td></tr>
<tr><td>5</td></tr>
<tr><td rowspan="5">3</td><td rowspan="5">14</td><td rowspan="5">59.6</td><td>1</td></tr>
<tr><td>2</td></tr>
<tr><td>3</td></tr>
<tr><td>4</td></tr>
<tr><td>5</td></tr>
</table>

Table 1: Information on filaments observed in experiments and the parameters used in the simulation.

## 3 Comparisons of velocity fields around filaments

In figures 1, 2, 3 and 4 we show the comparisons of calculated and experimentally measured velocity fields and their difference around four filaments, from filament 0 to filament 3 respectively, for sevral magnetic field frequences $f$. For easier comparison, velocity fields are scared with $2\omega L$ (where $\omega = 2\pi f$) and showed with logarithmic scale, while coordinates are normalized with filament length $L$.

## 4 Line integral of the azimuthal and radial velocity components

Figures 5, 6 and 7 show the line integrals of the azimuthal and radial velocity components around circular contours of radius r centered around origin for Filaments 1, 2 and 3 respectively. The solid lines correspond to simulations, $\times$ correspond to experiments and the dashed lines are the experimental moving average to help guide the eye.

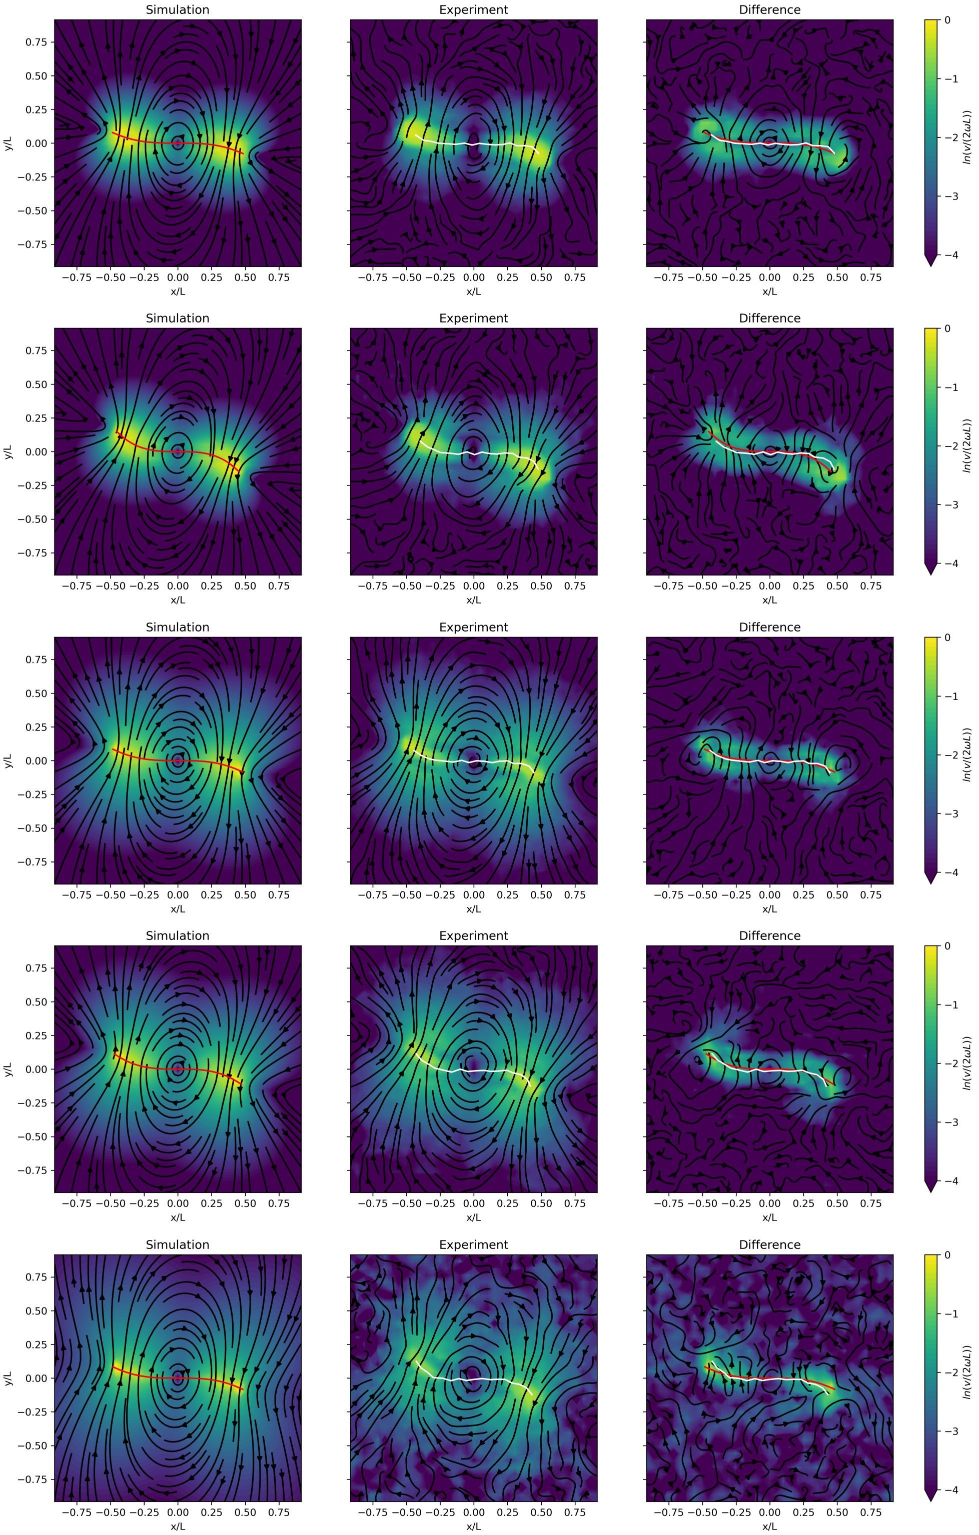


Figure 1: Velocity field around filament 0 for $f = 1$ Hz to 5 Hz starting from top to bottom.

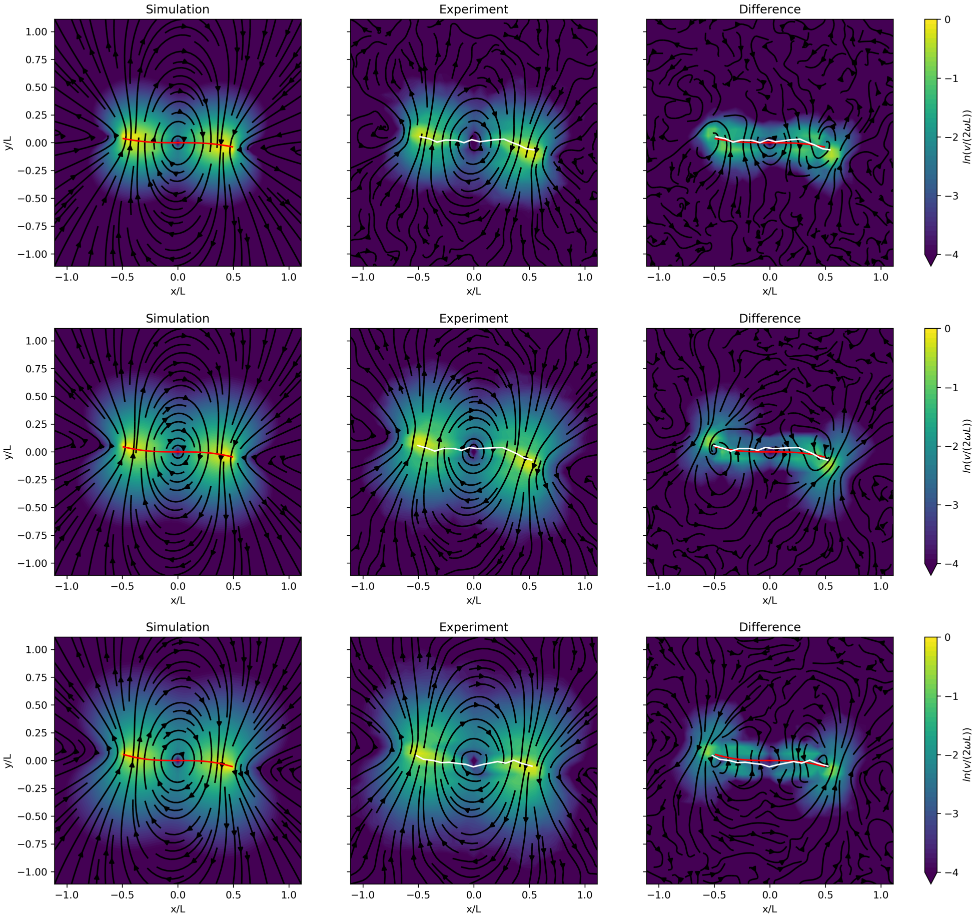


Figure 2: Velocity field around Filament 1 for $f = 1$ Hz to 3 Hz starting from top to bottom.

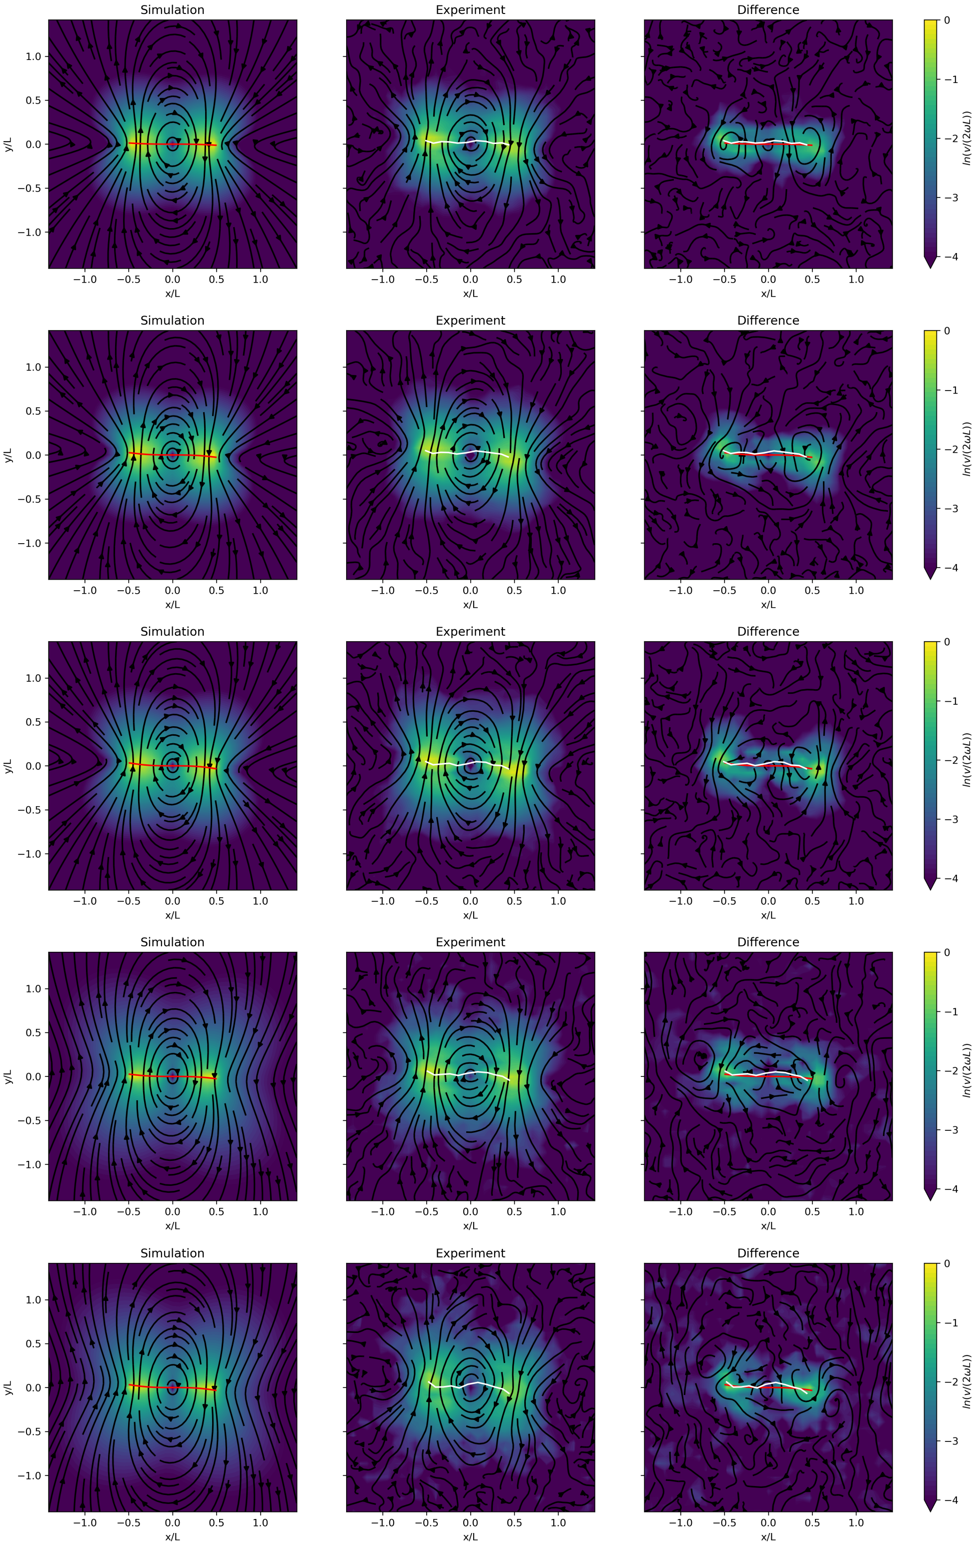


Figure 3: Velocity field around Filament 2 for $f = 1$ Hz to 5 Hz starting from top to bottom.

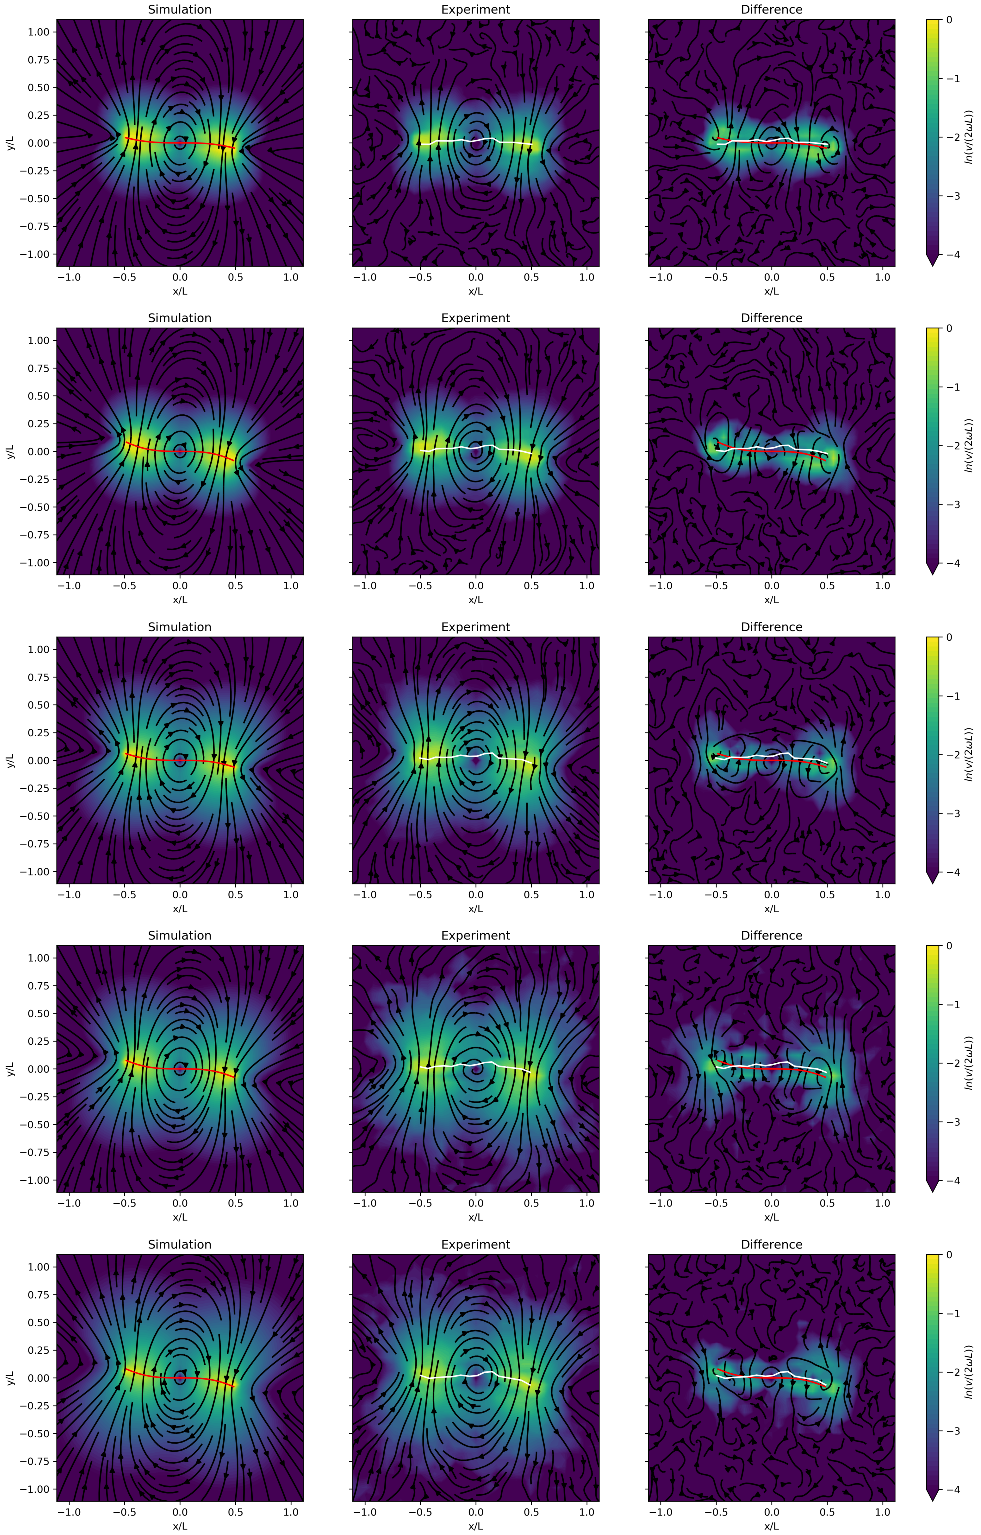


Figure 4: Velocity field around Filament 3 for $f = 1$ Hz to 5 Hz starting from top to bottom.

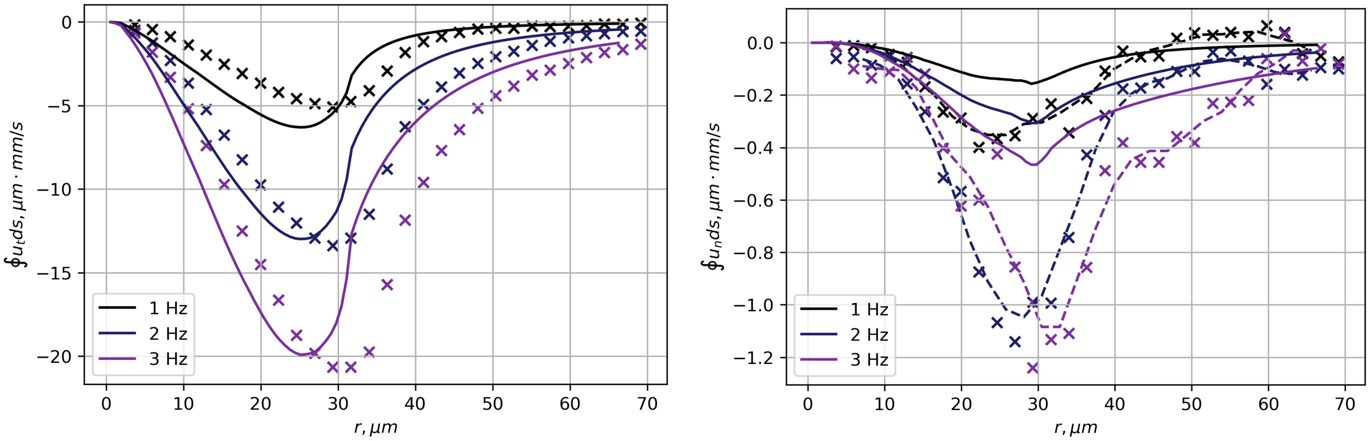


Figure 5: Line integral of the azimuthal (left) and radial (right) velocity components for Filament 1.

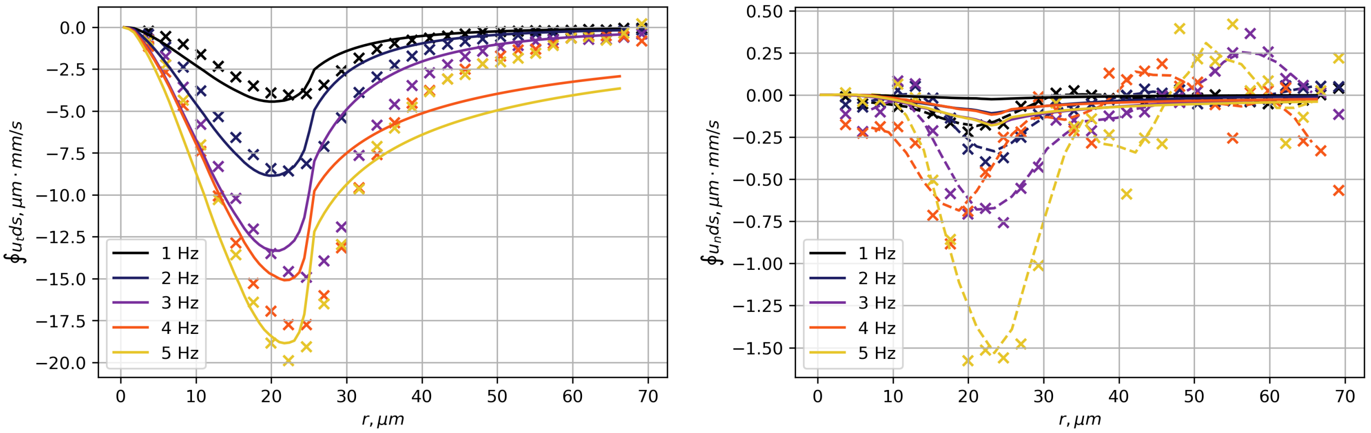


Figure 6: Line integral of the azimuthal (left) and radial (right) velocity components for Filament 2.

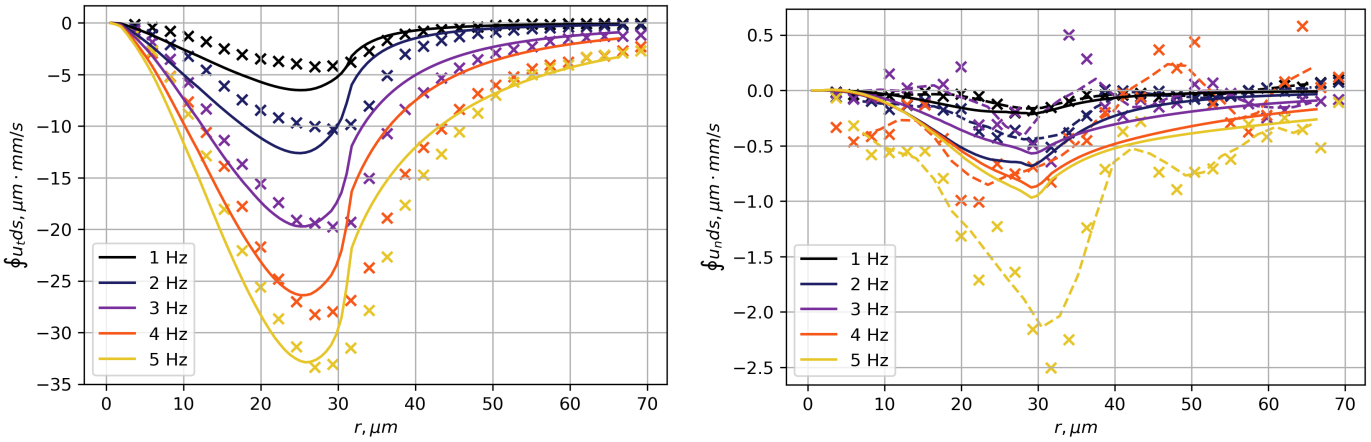


Figure 7: Line integral of the azimuthal (left) and radial (right) velocity components for Filament 3.
